# Supplementary material for: Exploring interlayer coupling in the twisted bilayer PtTe$_{2}$
Source: arXiv:2404.12461 source file (2024-04-18)
Supplement: Supplementary file 1 [file Supplemental_Material.pdf]

# Exploring interlayer coupling in the twisted bilayer $PtTe_2$ : Supplemental Material

Jeonghwan Ahn†,[1] Seoung-Hun Kang†,[1] Mina Yoon,[1] and Jaron T. Krogel[1,*]

*[1]Materials Science and Technology Division,*

*Oak Ridge National Laboratory, Oak Ridge, Tennessee 37831, USA*†

(Dated: April 17, 2024)

[*]Electronic address: krogeljt@ornl.gov

†These authors contributed equally to this work.

# I. FINITE-SIZE CORRECTION TO DMC SUPERCELL ENERGIES

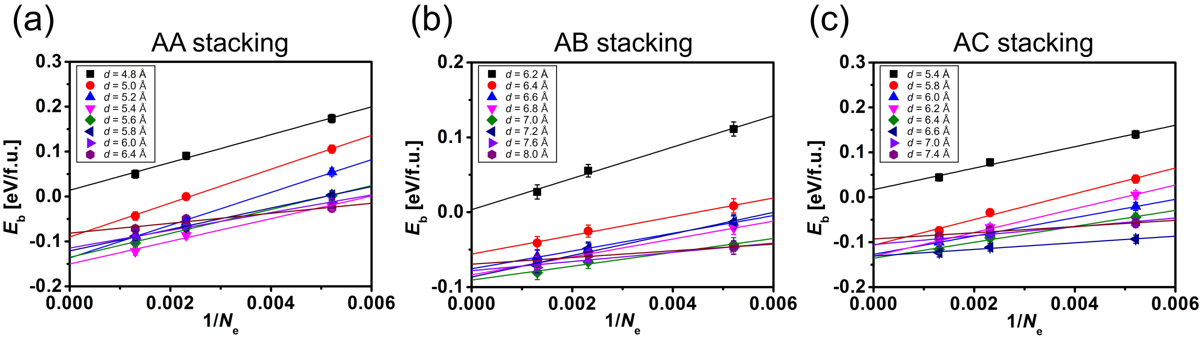


FIG. 1: DMC interlayer binding energies of the (a) AA-, (b) AB-, and (c) AC-stacked bilayer $PtTe_2$ at various interlayer distances as a function of $1/N_e$, where $N_e$ represents the total number of electrons in the supercell. Statistical errors are smaller than the symbol sizes. The solid lines in (a)-(c) represent an extrapolation through a linear fit.

## II. SUMMARY OF INTERLAYER BINDING ENERGIES AND SEPARATION DISTANCES COMPUTED WITH DMC AND DFT

TABLE I: Interlayer binding energies computed with DMC and DFT based on several different vdW functionals for the high symmetry bilayer $PtTe_2$ . The unit is in meV/Å$^2$.

| | DMC | $r^2$SCAN+rVV10 | $r^2$SCAN+D3 | $r^2$SCAN+MBD | PBE+D3 | PBE+MBD | vdW-optB86b | rev-vdW-DF2 | rVV10 | vdW-optB88 | vdW-DF2 |
|---|---|---|---|---|---|---|---|---|---|---|---|
| AA | 21(1) | -22 | -18 | -15 | -40 | -24 | -30 | -28 | -44 | -27 | -15 |
| AB | -13(1) | -11 | -11 | -8 | -17 | -8 | -14 | -12 | -22 | -14 | -11 |
| AC | -19(1) | -18 | -17 | -14 | -28 | -15 | -22 | -20 | -36 | -21 | -15 |

TABLE II: Interlayer separations computed with DMC and DFT based on several different vdW functionals for the high symmetry and the 21.79° twisted bilayer $PtTe_2$ along with the bulk $PtTe_2$. The unit is in Å.

| | DMC | $r^2$SCAN+rVV10 | $r^2$SCAN+D3 | $r^2$SCAN+MBD | PBE+D3 | PBE+MBD | vdW-optB86b | rev-vdW-DF2 | rVV10 | vdW-optB88 | vdW-DF2 |
|---|---|---|---|---|---|---|---|---|---|---|---|
| AA | 5.41(5) | 5.35 | 5.40 | 5.36 | 5.13 | 5.22 | 5.27 | 5.28 | 5.34 | 5.39 | 6.26 |
| AB | 7.02(6) | 6.95 | 6.98 | 7.03 | 6.66 | 6.80 | 6.78 | 6.82 | 6.65 | 6.80 | 7.07 |
| AC | 6.27(5) | 6.18 | 6.22 | 6.26 | 5.73 | 5.87 | 5.85 | 5.85 | 5.83 | 6.15 | 6.53 |
| 21.79° | 6.52(6) | 6.47 | 6.53 | 6.42 | 6.02 | 6.24 | 6.21 | 6.22 | 6.09 | 6.31 | 6.70 |
| Bulk | 5.27(3) | 5.30 | 5.36 | 5.36 | 5.05 | 5.19 | 5.24 | 5.25 | 5.28 | 5.35 | 5.85 |

## III. BAND STRUCTURES DEPENDING ON THE STACKING MODE

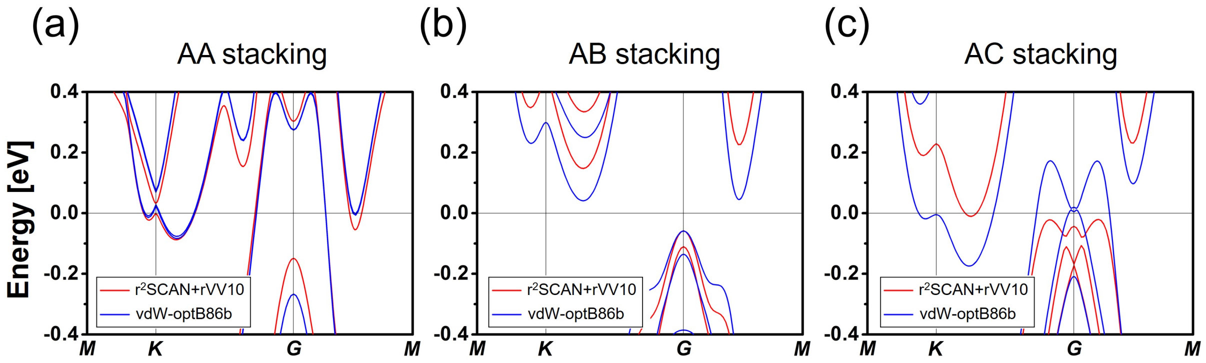


FIG. 2: The comparison of between the band structures computed with $r^2$SCAN+rVV10 (red) and vdW-optB86b for (a) AA-, (b) AB-, and (c) AC-stacked bilayer $PtTe_2$ with inclusion of spin-orbit coupling.
